# Supplementary material for: All-charm tetraquark mass and possible quantum numbers of X(6900)
Source: arXiv:2309.04794 source file (2023-09-09)
Supplement: Supplementary file 1 [file Supplemental_file_1.pdf]

```
(*The code based on the code written by Schloberl and published in
  "Solving the Schrodinger equation for bound states with Mathematica 3.0"
  by Lucha and Schloberl .
   The code was first used in our (Morgan Kuchta) Bachelor 's thesis .
   Original code that uses Runge-Kutta method can be found in the referenced text.
   We modified the code for the newer versions of the Mathematica ,
provided additional comments to the original code and adapting to Mathematica 12,
added functions "Pair" and "Pair2" and "PairTable". Code can be easily
  adjusted for any type of potential that allows for reasonable cut-off.
   "Pair" functions generate apropriate terms in the Hamiltonian and
  Cornell potentail . Pair 2 uses simplified results for the tensor term.
*)

(* MinFind - Finds minimum potential to the right:
      RightB - righ border
      Step - Size of the step
      Minimum - minimum
      Low - lower bound
      Upp - upper bound
      Nod - number of nodes
      Feh - error of energy
      m1,m2,m3,m4 - masses of quarks
      mu12, mu34 - reduced masses of cluseters
      mu1234 - total reduced mass
      l12,l34 - orbital excidation of pairs
      l1234 - total orbital excitation
      V[] - Various potentials
      h - integration stepsize
*)
```

```
In[ ]:= MinFind[l1_, h1_, Step_, RightB_, ww1_] :=
  Module[{l = l1, h = h1, step = Step, right = RightB, ww = ww1},
        del = h / 10;
        xs = right;
        If[xs < del, Goto[TooSmall]];
   (* Checks of minimum to the right isn't too small *)
        If[l < 1, Goto[3]];
        Label[Loop1];
        If[xs < step + del, xs = del; Goto[2]];
        ms = ww * vl[xs] + l * (l + 1) / xs ^ 2;
        rs = ww * vl[xs + step] + l * (l + 1) / (xs + step) ^ 2;
        ls = ww * vl[xs - step] + l * (l + 1) / (xs - step) ^ 2;
        If[rs > ms && ms > ls, xs = xs - step; Goto[Loop1]];
        If[rs < ms && ls > ms, xs = xs + step; Goto[Loop1]];
        If[rs == ls , Goto[2]];
        If[rs > ms && ls > ms, If[step < h, Goto[2]];
    step = step / 10;
    Goto[Loop1]];
        Print["SOMETHING  IS WRONG , ANALYZE  POTENTIAL  "];
        Goto[10];
        Label[3];
        Label[Loop2];
        If[xs < step + del, xs = del; Goto[2]];
        ms = ww * vl[xs];
   rs = ww * vl[xs + step];
        ls = ww * vl[xs - step];
        If[rs > ms && ms > ls, xs = xs - step; Goto[Loop2]];
        If[rs < ms && ls > ms, xs = xs + step; Goto[Loop2]];
        If[rs == ls , Goto[2]];
        If[rs > ms && ls > ms, If[step < h, Goto[2]];
    step = step / 10;
    Goto[Loop2]];
        Print["SOMETHING  IS WRONG , ANALYZE  POTENTIAL "];
        Goto[10];
        Label[TooSmall];
        Print["XMIN  TOO  SMALL "];
        Goto[10];
        Label[2];
        Minimum = xs;
        Label[10];
        Clear[xs, ww];
        Return[Minimum]]

(*Two  functions  for solving  Schodinger  equation . Identical  except  some
  parameters  in MinFind  and  integration  limits . Function  Schrodinger2  was
  used  in Pair  2 function  and while  Schrodinger  was used  in Pair  function . *)

In[ ]:= Schrodinger[Low_, Upp_, Nod_, l1_, h1_, m1_, m2_] :=
  Module[{low = Low * ww, upp = Upp * ww, nod = Nod, l = l1, h = h1, w1 = m1, w2 = m2},
```

```
 (*
 This parts finds minimum tu the right
  *)
   ww = 2 w1 * w2 / (w1 + w2);
   Mini = MinFind[l, h, 0.01, 5, ww];
   Mini = Mini + h;
   del = h / 10;
   Feh = 0.00001 * ww;
       (* Defining diffl = Veff - e, y'' = (Veff - e)y *)
   diffl[xxx_, l_, een_] := ww * vl[xxx] + l * (l + 1) / xxx ^ 2 - een;
Label[Start];
        seh = upp - low;
        eps = (low + upp) / 2;
       (*
 Starting the integration with the boundaries y(del) = del^(l+1),
 y'(del) = (l+1)del^l and with the energy eps equal to the arithmetic mean
   of the preceding lower and upper bounds of energy low and upp
 *)
        x = del;
        y = x ^ (l + 1);
        yp = (l + 1) * x ^ l;
        yold = 1;
        n0x = 0;
       (*
 If the desired accuracy (prescribed error Feh) has been obtained ,
 the bound state energy is taken as the arithmetic mean of the last low and upp
 *)
       If[seh < Feh, Goto[1]];
       (*
 Integrating y'' = (Veff - e)y one step h further with the Runge - Kutta method
 *)
   Label[2];
        a1 = yp * h; b1 = diffl[x, l, eps] * h * y;
 a2 = (yp + b1 / 2) * h;
 hh = diffl[x + h / 2, l, eps] * h;
                  b2 = hh * (y + a1 / 2);
 a3 = (yp + b2 / 2) * h;
 b3 = hh * (y + a2 / 2); a4 = (yp + b3) * h;
        x = x + h; u2 = diffl[x, l, eps]; b4 = u2 * h * (y + a3);
              y = y + (a1 + 2 * a2 + 2 * a3 + a4) / 6;
           yp = yp + (b1 + 2 * b2 + 2 * b3 + b4) / 6;
       (*
 Counting the number of nodes by n0x until the prescribed n0 is reached
 *)
           If[y * yold > 0, Goto[3]];
           n0x = n0x + 1;
```

```
          If[n0x > nod , Goto[4]];
Label[3];
       yold = y;
       (*
If the following condition is not fullfilled ,
x is greater then the classical turning point *)
          If[(u2 < 0 || x < Mini), Goto[2]];
       (*
If (after stating that x greater then the classical turning point) y*yp is greater
than 0 (i.e. y and yp have the same sign), one is sure that y goes to infinity
   without having additional nodes. Otherwise one has to integrate further
*)
       z = y * yp;
          If[z < 0, Goto[2]];
       (*
If y goes to infinity , a new el is established by eps.
*)
       low = eps;
          Goto[Start];
       (*
If nox exceeds n0, a new eu is established by eps
*)
    Label[4];
       upp = eps;
          Goto[Start];
       (*
In the following lines the wave function y is calculated using the above
 calculated bound
state energy (the last eps) by the same method as above. In addition y
 is stored in feld1
at x which is stored in xcoord,
and the number of integration steps is counted by j.
*)
Label[1];
          ep = eps;
       j = 0;
 Label[20];
             j = j + 1;
                feld1[j] = y;
             xcoord[j] = del + (j - 1) * h;
             j1 = j;
             xmax = xcoord[j1];
       (*
Integrating y'' = (Veff - e)y one step h further with the Runge - Kutta method
*)
       a1 = yp * h;  b1 = diffl[x, l, eps] * h * y;
```

```
a2 = (yp + b1 / 2) * h;
hh = diffl[x + h / 2, l, eps] * h;
            b2 = hh * (y + a1 / 2);
a3 = (yp + b2 / 2) * h;  b3 = hh * (y + a2 / 2);
a4 = (yp + b3) * h;
      x = x + h; u2 = diffl[x, l, eps]; b4 = u2 * h * (y + a3);
            y = y + (a1 + 2 * a2 + 2 * a3 + a4) / 6;
         yp = yp + (b1 + 2 * b2 + 2 * b3 + b4) / 6;
            If[y * yold > 0, Goto[30]];
      n0x = n0x + 1;
               If[n0x > nod , Goto[40]];
Label[30];
            yold = y;
         If[(u2 < 0 || x < Mini ), Goto[20]];
      z = y * yp;
      If[z < 0, Goto[20]];
Label[40];
          (*
The  reduced  radial  wave  function  yschr  obtained  from  the  interpolation
 of  the  data  stored  in  feld1  and  in  xcoord
*)
            yschr  = Interpolation [Table[{xcoord[j], feld1[j]}, {j, 1, j1}]];
           xmax = xcoord[j1];
NoNorm  = NIntegrate [yschr[x]^2, {x, del , 5}];
Distance  = NIntegrate [1/NoNorm * x * yschr[x]^2, {x, del , 5}];
    (*
 Output  of  the  resulting  norm ,  averange  value  of  x,  max  of  x,  and  disctan
*)
Return[{N[ep / ww, 10], NoNorm , Distance }];
  Clear[NoNorm , Distance , xmax , yschr ]]
Schrodinger2 [Low_ , Upp_ , Nod_ , l1_ , h1_ , m1_ , m2_] :=
Module[{low = Low * ww, upp = Upp * ww, nod = Nod , l = l1, h = h1, w1 = m1, w2 = m2},

  ww = (2 w1 * w2) / (w1 + w2);
  Mini = MinFind[l, h, 0.001 , 10 , ww];
  Mini  = Mini + h;
  del  = h / 10;
  Feh = 0.00001 * ww;

  diffl[xxx_ , l_, een_] := ww * vl[xxx] + l * (l + 1) / xxx ^ 2 - een;
Label[Start];
       seh = upp - low;
       eps = (low + upp) / 2;

  x = del;
```

```
        y = x^(l + 1);
        yp = (l + 1) * x^l;
        yold = 1;
        n0x = 0;

        If[seh < Feh, Goto[1]];

    Label[2];
        a1 = yp * h; b1 = diffl[x, l, eps] * h * y;
 a2 = (yp + b1 / 2) * h;
 hh = diffl[x + h / 2, l, eps] * h;
                 b2 = hh * (y + a1 / 2);
 a3 = (yp + b2 / 2) * h;
 b3 = hh * (y + a2 / 2); a4 = (yp + b3) * h;
        x = x + h; u2 = diffl[x, l, eps]; b4 = u2 * h * (y + a3);
              y = y + (a1 + 2 * a2 + 2 * a3 + a4) / 6;
           yp = yp + (b1 + 2 * b2 + 2 * b3 + b4) / 6;



           If[y * yold > 0, Goto[3]];
           n0x = n0x + 1;
           If[n0x > nod, Goto[4]];
Label[3];
       yold = y;

           If[(u2 < 0 || x < Mini), Goto[2]];

       z = y * yp;
           If[z < 0, Goto[2]];

       low = eps;
           Goto[Start];

    Label[4];
       upp = eps;
           Goto[Start];

 Label[1];
           ep = eps;
       j = 0;
 Label[20];
              j = j + 1;
                 feld1[j] = y;
              xcoord[j] = del + (j - 1) * h;
              j1 = j;
              xmax = xcoord[j1];
```

```
        a1 = yp * h;  b1 = diffl[x, l, eps] * h * y;
  a2 = (yp + b1 / 2) * h;
  hh = diffl[x + h / 2, l, eps] * h;
              b2 = hh * (y + a1 / 2);
  a3 = (yp + b2 / 2) * h; b3 = hh * (y + a2 / 2);
  a4 = (yp + b3) * h;
        x = x + h; u2 = diffl[x, l, eps]; b4 = u2 * h * (y + a3);
              y = y + (a1 + 2 * a2 + 2 * a3 + a4) / 6;
           yp = yp + (b1 + 2 * b2 + 2 * b3 + b4) / 6;
              If[y * yold > 0, Goto[30]];
        n0x = n0x + 1;
                 If[n0x > nod, Goto[40]];
  Label[30];
              yold = y;
           If[(u2 < 0 || x < Mini), Goto[20]];
        z = y * yp;
        If[z < 0, Goto[20]];
  Label[40];

              yschr = Interpolation[Table[{xcoord[j], feld1[j]}, {j, 1, j1}]];
              xmax = xcoord[j1];
  NoNorm = NIntegrate[yschr[x]^2, {x, del, 10}];
  Distance = NIntegrate[1/NoNorm * x * yschr[x]^2, {x, del, 10}];

Return[{N[ep / ww, 10], NoNorm, Distance}];
  Clear[NoNorm, Distance, xmax, yschr]]

(*Pair Function creates Cornell potential with Spin-
 Spin interation and solves SE for two Quarks*)
(*Inputs :
 1-Strong coupling constant , 2- string tension ,
3-Cassimir coeff . 4. Sigma for Spin-Spin ,
5-8 Quantum numbers 9-10 Masses*)

In[ ]:= Pair[Alpha_, Be_, KappaS_, Sigma_, S_, L_, J_, Nod_, M1_, M2_] :=
 Module[{a = Alpha, b = Be, k = KappaS, sig = Sigma, s = S, l = L, j = J, nod = Nod,
    m1 = M1, m2 = M2},
  mu = (m1 * m2)/(m1 + m2);
  (* First Spin dependent term*)
  If[s == 0, Goto[10], Goto[20]];
  Label[10];
    ss = -3/4;
```

```
Goto[EndS1];
Label[20];
If[s == 1, Goto[30], Goto[Error]];
Label[30];
ss = 1/4;
Goto[EndS1];
Label[EndS1];
(*Second Spin Dependent Term*)
If[l == 0, sl = 0; t = 0; Goto[EndS3]];
If[l < 0, Goto[Error]];
If[j == l - 1, Goto[L1]];
If[j == l, Goto[L2]];
If[j == l + 1, Goto[L3]];
Label[L1];
sl = -(l + 1);
Goto[EndS2];
Label[L2];
sl = -1;
Goto[EndS2];
Label[L3];
sl = l;
Goto[EndS2];
Label[EndS2];
(*Third Spin Dependent Term*)
If[j == l, Goto[T1]];
If[j == l - 1, Goto[T2]];
If[j == l + 1, Goto[T3]];
Label[T1];
t = 2;
Goto[EndS3];
Label[T2];
t = -2 (l + 1) / (2 l - 1);
Goto[EndS3];
Label[T3];
t = -2 l / (2 l + 3);
Goto[EndS3];
Label[EndS3];
(*End of Spin dependent terms*)
(*Checking for errors*)
If[m1 < 0, Goto[Error]];
If[m2 < 0, Goto[Error]];
If[nod < 0, Goto[Error]];
(*End of checking for errors*)
```

```
vl[x_] := - (8 k * a * Pi)/(3 mu^2) (sig/Sqrt[Pi])^3 Exp[- sig^2 * x^2] ss + k a/x + b * x;
Scho = Schrodinger [-1, 3, nod , l, 0.1 , m1 , m2];
Dis = Scho[[3]];
A = -((3 k * a)/(2 * mu^2) * 1/Dis^3 + b/(2 mu^2) * 1/Dis) sl;
B = - (3 k * a)/mu^2 * 1/Dis^3 t;
Result = Part[Scho , 1] + A + B + m1 + m2 ;
Goto[Finish ];
Label [Error ];
Print ["SOMETHING  IS  WRONG , ANALYZE  POTENTIAL "];
Goto[Finish ];
Label[Finish ];
Return [{Result , A, B, Dis }];
Clear [A, B, Scho]
]
(*Solves  SE  for  two  pairs .  1-4  see  above ,  5-mass  of  the  foce  carrier ,
6-13  quantum  numbers  ,  14-15  masses  *)
Pair2[Alpha_ , Be_ , KappaS_ , Sigma_ , Mi_ , S1_ , S2_ , S_ , LL1_ , LL2_ , LL_ , J_ ,
  Nod_ , M1_ , M2_] :=
 Module [{a = Alpha , b = Be , k = KappaS , sig = Sigma , mi = Mi , s1 = S1 , s2 = S2 ,
    spin = S, l1 = LL1 , l2 = LL2 , l = LL , j = J, nod = Nod , m1 = M1 , m2 = M2},
  mu = (m1 * m2)/(m1 + m2);
  pip = 0;
  (* First  Spin  dependent  term*)
  If[spin == 0, Goto [S10] ];
  If[spin == 1, Goto [S20]];
  If[spin == 2, Goto [S30]];
  Label [S10];
  If[s1 == 0 && s2 == 0, Goto [S11], Goto [S12]];
  Label [S11];
  ss = 0; sl = 0; t = 0; Goto [EndS3 ];
  Label [S12];
  If[s1 ≠ 1, Goto [Error ]];
  If[s2 ≠ 1, Goto [Error ]];
  ss = -2; sl = 0; t = 0; Goto [EndS3 ];
  Label [S20];
  If[s1 == 1 && s2 == 1, Goto [S21], {ss = 0, Goto [EndS1 ]} ];
  Label [S21];
  ss = -1; pip = 1; Goto [EndS1 ];
  Label [S30];
  If[s1 ≠ 1 && s2 ≠ 1, Goto [Error ]];
```

```
ss = 1; pip = 1;
Label[EndS1];
If[l == 0, {sl == 0, t == 0, Goto[EndS3]}];
If[l < 1, Goto[Error]];
If[spin == 1, Goto[L40], Goto[L50]];
Label[L40];
If[j == l - 1, {sl = -(l - 1), Goto[EndS2]}];
If[j == l, {sl = -1, Goto[EndS2]}];
If[j == l + 1, {sl = l, Goto[EndS2]}, Goto[Error]];
Label[L50];
If[j == l - 2, {sl = -2 l - 2, Goto[EndS2]}];
If[j == l - 1, {sl = -(l + 3), Goto[EndS2]}];
If[j == l, {sl = -3, Goto[EndS2]}];
If[j == l + 1, {sl = l - 2, Goto[EndS2]}];
If[j == l + 2, {sl = 2 l, Goto[EndS2]}, Goto[Error]];
Label[EndS2];
If[pip == 0, {t = 0, Goto[EndS3]}];
If[l ≠ 1, {t = 0, Goto[EndS3]}];
If[j == spin - 1, {t = -8, Goto[EndS3]}];
If[j == spin, {t = 4, Goto[EndS3]}];
If[j == spin + 1, {t = -4/5, Goto[EndS3]}, Goto[Error]];
Label[EndS3];
(*Checking for errors*)
If[m1 < 0, Goto[Error]];
If[m2 < 0, Goto[Error]];
If[nod < 0, Goto[Error]];
(*End of checking for errors*)
vl[x_] := -(8 k*a*Pi)/(3 mu^2) (sig/Sqrt[Pi])^3 Exp[-sig^2*x^2] ss + k a/x Exp[-mi*x] + x*b;
(*Feel free to change felt and right limit or add dependence on vl. Method
 used here is the fastest of the ones I tested.*)
LimL = -1; LimR = 5;
Scho = Schrodinger2[LimL, LimR, nod, l, 0.01, m1, m2];
Dis = Scho[[3]];
A = -((3 k*a)/(2*mu^2) * 1/Dis^3 + b/(2 mu^2) * 1/Dis) sl;
B = -(3 k*a)/mu^2 * 1/Dis^3 * t;
Result = Part[Scho, 1] + A + B + m1 + m2;
Goto[Finish];
Label[Error];
Print["SOMETHING IS WRONG, ANALYZE INPUT"];
Goto[Finish];
```

```
  Label[Finish ];
  Return [{Result , A, B, Dis }];
  Clear [A, B, Scho , ss]
 ]

(*Other  useful  functions
  Pair  Table  maskes  the  table .)
```

In[ ]:=
```
PairTable [Alpha_ ,  Beta_ ,  KappaS_ ,  Sigma_ , SM_ , LM_ , NM_ ,  M1_ , M2_] :=
 Module [{a = Alpha ,  b = Beta ,  k = KappaS ,  sig = Sigma , sm = SM , lm = LM , nm = NM ,
   m1 = M1 , m2 = M2},
  Table [Table [Pair [a, b, k, sig , sm , L, J, Node , m1 , m2][[1]], {Node , 0, nm},
    {J, Abs[sm - L], sm + L}], {L, 0, lm}]]


(*Strong  is  used  for  the  calculation  of  alpha_s . *)

Strong [A_ , B_] := Module [{a = A * 1000 , b = B * 1000 }, 3.252373534 / Log[(((a * b) / (a + b)) ^ 2) / 0.112 ^ 2]]
```
